# Supplementary material for: Evolution of a Modular Software Network
Source: arXiv:1111.5251 source file (2011-11-22)
Supplement: Supplementary file 1 [file supplementary.pdf]

# The Evolution of a Modular Software Network

Miguel A. Fortuna[*], Juan A. Bonachela, and Simon A. Levin

Department of Ecology and Evolutionary Biology
Princeton University, 08544 Princeton, New Jersey, USA

## SUPPLEMENTARY INFORMATION

The Debian project was born in 1993. Since then, eleven stable versions have been released to date, all of them named after a character in the movie Toy Story (Buzz (1996), Rex (1996), Bo (1997), Hamm (1998), Slink (1999), Potato (2000), Woody (2002), Sarge (2005), Etch (2007), Lenny (2009), and Squeeze (2011)). In this study we have compiled the binary i386 packages, along with their dependencies and conflicts of the first ten releases (from Buzz to Lenny). They were downloaded from http://archive.debian.org/debian/dists/. The files (in txt format) are available from the website of this journal as a zip folder.

[*]To whom correspondence should be addressed. E-mail: fortuna@ebd.csic.es, Phone: +34 954 621 125

# Table I.

## Description of the components of the interaction network of Debian GNU/Linux over time

(release, release name, release date, number of packages, number of packages with interactions, number of dependencies, number of conflicts, number of packages with outgoing dependencies, number of packages with outgoing conflicts, number of packages with incoming dependencies, and number of packages with incoming conflicts)

| **Release** | **Codename** | **Year** | **Packages** | **Inter_Pack** | **Dependencies** | **Conflicts** | **Pack_**$k_{out}^{dep}$ | **Pack_**$k_{out}^{con}$ | **Pack_**$k_{in}^{dep}$ | **Pack_**$k_{in}^{con}$ |
|---|---|---|---|---|---|---|---|---|---|---|
| 1.1 | Buzz | 1996 | 488 | 379 | 539 | 28 | 351 | 27 | 91 | 22 |
| 1.2 | Rex | 1996 | 738 | 633 | 943 | 29 | 596 | 26 | 138 | 23 |
| 1.3 | Bo | 1997 | 1126 | 984 | 1744 | 62 | 936 | 56 | 212 | 53 |
| 2.0 | Hamm | 1998 | 1852 | 1677 | 3631 | 199 | 1603 | 166 | 398 | 140 |
| 2.1 | Slink | 1999 | 2664 | 2395 | 5983 | 336 | 2293 | 257 | 591 | 237 |
| 2.2 | Potato | 2000 | 4305 | 3851 | 10617 | 632 | 3631 | 456 | 1310 | 413 |
| 3.0 | Woody | 2002 | 8747 | 8040 | 28225 | 1687 | 7771 | 1100 | 2782 | 1062 |
| 3.1 | Sarge | 2005 | 15658 | 14657 | 66125 | 3148 | 14065 | 2034 | 5917 | 1783 |
| 4.0 | Etch | 2007 | 23159 | 18632 | 90213 | 4530 | 16714 | 2763 | 7485 | 2946 |
| 5.0 | Lenny | 2009 | 28245 | 22919 | 101521 | 4755 | 20768 | 3011 | 9495 | 3273 |

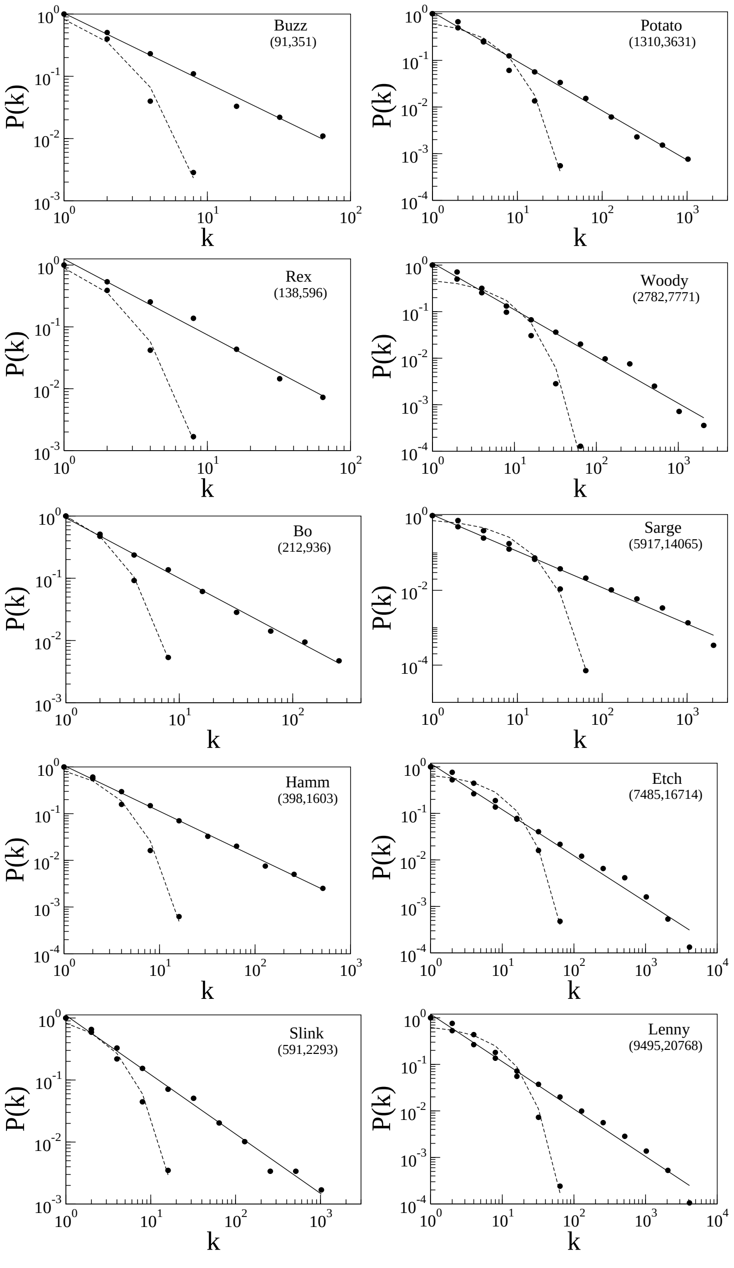


**Figure 1:** *Cummulative degree distribution of the number of incoming (solid lines) and outgoing (dashed lines) dependencies for the software packages of the first ten releases of the Debian GNU/Linux operating system (from top to bottom and from left to right). The figures depict the probability, P(k), for a package to depend on or to be needed by at least, 1, 2, 3, ..., k packages to work. Both axes are in logarithmic scale. In every release the best fit for the outgoing dependencies is an exponential function while for the incoming dependencies is a power-law. Inset, the number of packages with incoming or outgoing dependences (in parenthesis, respectively) and the name of the release are indicated.*

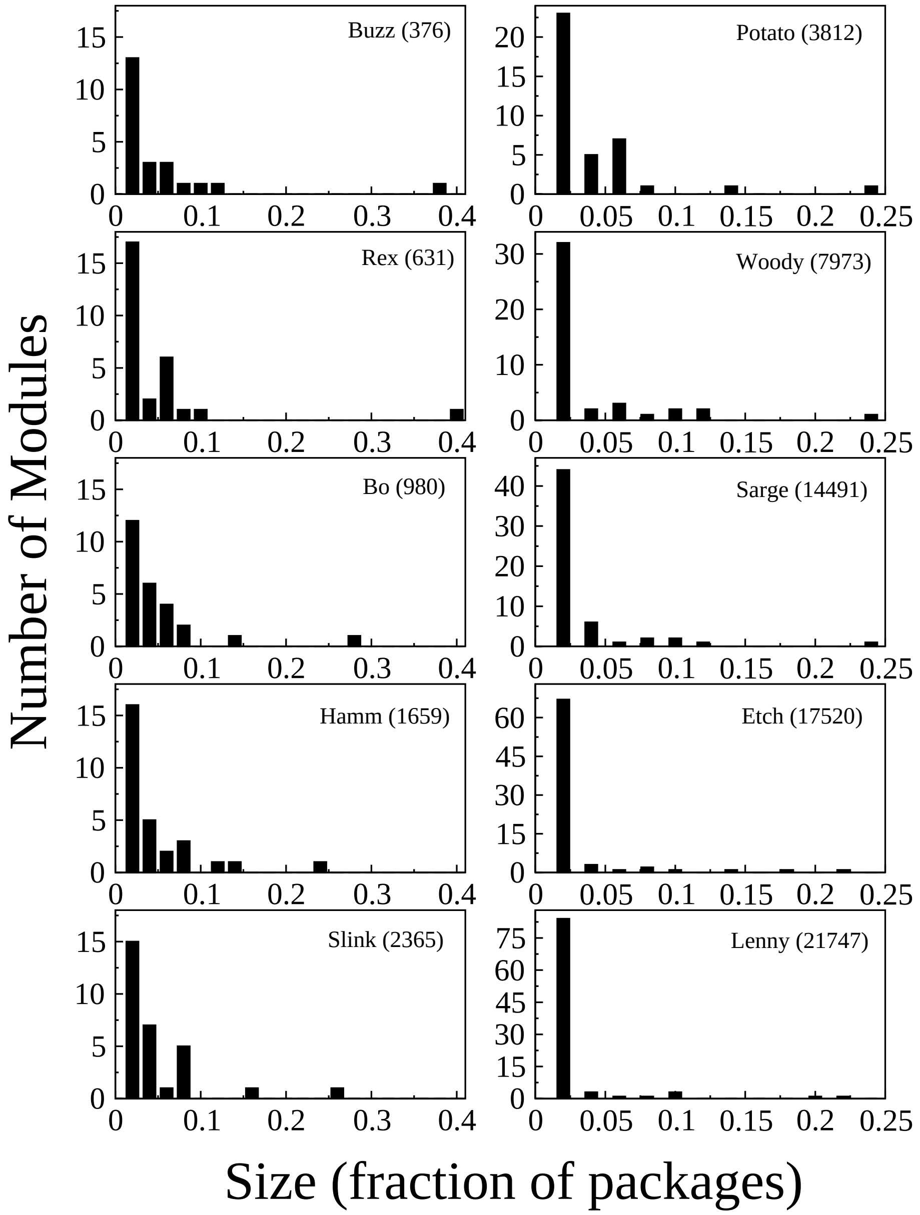


**Figure 2:** *Distribution of the size of the modules identified by the modularity algorithm for each release of the Debian GNU/Linux operating system (release name and total number of interacting packages inside each plot). The first five releases (on the left) consist of approximately the same number of modules (between 23 and 30). In the successive releases (on the right) the number of modules increased over time (until 94 for the most recent version). However, the size of most modules was smaller over time in relation to the total number of interdependent packages constituting each release. The number of modules consisting of at least 5% of the total number of interdependent packages oscillated between 6 and 8 for all releases.*

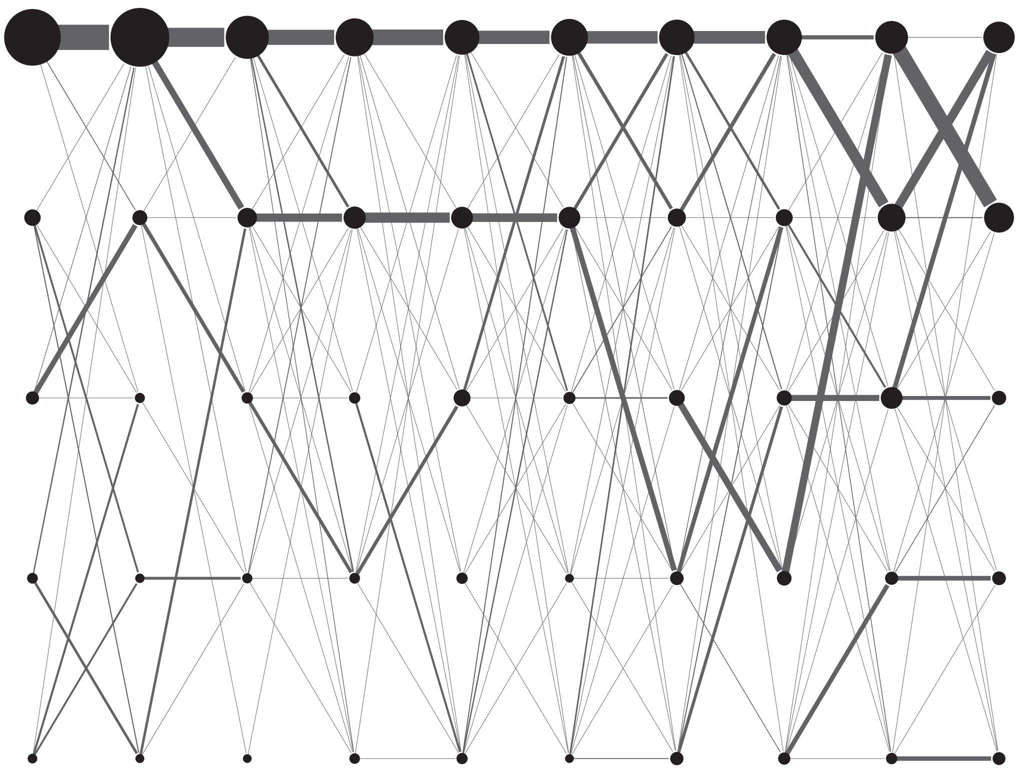

**Figure 3:** *Schematic representation of the fate of the modules of interdependent packages along the first ten releases of the Debian GNU/Linux operating system. Nodes along each column represent the five largest modules of each release, and their size is proportional to the number of packages constituting each release. The thickness of the line between two nodes indicates the fraction of packages from one module in one release that are assigned to another module in the next release (from left to right). Most nodes only have one thick line in each direction, meaning that the packages constituting the largest modules do not tend to break up themselves in several modules in the next release, but to keep together as one component of the new module.*

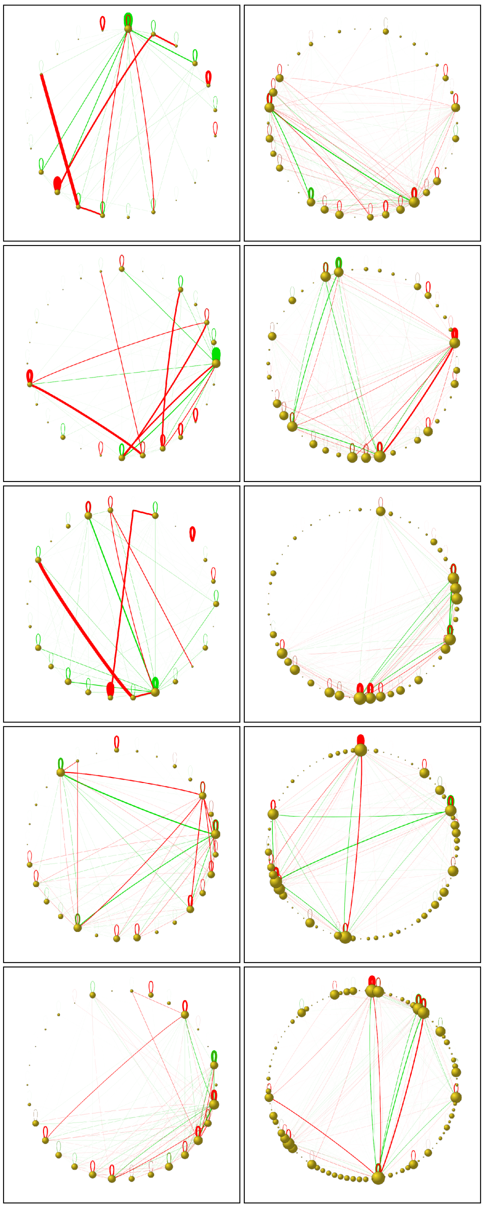

**Figure 4:** *Evolution of the modularity in a software network. The modular structure of the first ten releases of the Debian GNU/Linux operating system are represented (from top to bottom and from left to right). Nodes in each plot depict modules and links indicate the fraction of dependencies (in green) and conflicts (in red) between packages assigned to different modules (or within modules, loops). The size of the nodes is proportional to the logarithm of the number of packages. The number of modules and the fraction of conflicts within modules increased over time while the fraction of dependencies within modules remained constant. (Note that red color can hide green color in the loops).*
